# Supplementary material for: Comparing Rule-based, Feature-based and Deep Neural Methods for De-identification of Dutch Medical Records
Source: arXiv:2001.05714 source file (2020-01-16)
Supplement: Supplementary file 1 [file 99-appendix.tex]

\appendix
\section{Supplemental Material}\label{sec:appendix}

\subsection{Annotation Guidelines}\label{sec:appendix-annotation-guidelines}
For the development of an automatic de-identification software, we require medical records where the protected health information (PHI) has been marked up so that the annotations can be used to develop automatic de-identification methods.
The annotated data is the type information that must be removed/replaced from a patient record in order to be considered de-identified.
We defined 8 categories of PHI that can relate to a patient, but also to relatives, employers, household members or the doctor of a patient.
In total 16 tags can be assigned to a piece of text:

\begin{enumerate}
  \setlength{\parskip}{0pt}
  \item NAME
  \begin{itemize}
    \item Name
    \item Initials
  \end{itemize}
  \item PROFESSION (not of medical staff)
  \item LOCATION
  \begin{itemize}
    \item Hospital
    \item Care Institute (Zorgorganisatie)
    \item Organization/Company
    \item Address
    \item Internal location (e.g., building code, room, floor)
  \end{itemize}
  \item AGE
  \item DATE
  \item CONTACT
  \begin{itemize}
    \item Phone/FAX
    \item Email
    \item URL/IP-address
  \end{itemize}
  \item ID
  \begin{itemize}
    \item Social security number (SSN/BSN)
    \item Any other ID number
  \end{itemize}
  \item OTHER
\end{enumerate}
\vspace{2cm}
\balance

\subsubsection{Overall Annotation Rules}
When annotating, the following rules apply:
\begin{enumerate}
  \setlength{\parskip}{0pt}
  \item When tagging something that is PHI but it is not obvious what to tag it as, think about what it should be replaced with and whether that will make sense in the document (``replacement test'').
  \item When in doubt whether something is \emph{tag A} or \emph{tag B}, annotate it as the most likely tag and add a note to the annotation.
  \item When in doubt, annotate! We do not want to miss PHI.
\end{enumerate}
To give an example of the replacement test, consider this sentence:
\begin{exmp}
  \emph{In 2015 is hij met de andere cliënten verhuisd naar de
  woonvoorziening Kerklaan in Bennebroek.}
  \\[0.2em] [Translated]
  \emph{In 2015 he moved with other clients to the
  housing facility Kerklaan in Bennebroek.}
\end{exmp}
\noindent
It is clear that the housing facility has been named after its location ``Kerklaan.'' So instead of
annotating ``Kerklaan'' as an address, ``housing facility Kerklaan'' should be annotated as care
institute, as we would replace this with the name of another care institute. The final annotation
should look like this:
\begin{exmp}
  \emph{In \textless DATE 2015\textgreater\ is hij met de andere cliënten verhuisd naar de
  \textless CARE-INSTITUTE woonvoorziening Kerklaan\textgreater\ in \textless ADDRESS Bennebroek\textgreater.}
  \\[0.2em]
  [Translated] \emph{In \textless DATE 2015\textgreater\ he moved with other clients to the
  \textless CARE-INSTITUTE housing facility Kerklaan\textgreater\ in \textless ADDRESS Bennebroek\textgreater.}
\end{exmp}

\subsubsection{Example Annotations per Category}
\cref{tab:example-annotations} provides example annotations for each of the PHI categories that were distributed to each annotator alongside with the instructions.

\begin{table*}[t]
\caption{Examples provided to the annotators alongside with the annotation instructions.}
\label{tab:example-annotations}
\resizebox{\textwidth}{!}{%
\begin{tabular}{@{}lp{.4\textwidth}p{.4\textwidth}@{}}
\toprule
Category & Examples & Exclude from Annotation \\ \midrule
Name & ``Bart van der Boor'', ``Boor, van der'', ``B. Boor'', ``Anne FP Jansen'' & Titles (Dhr., Mw., Dr., etc.) \\
Initials & J.F., JF. & Titles (see above) \\
Profession & ``stratenmaker'', ``programmeur'', ``militaire dienst'' & Professions of medical staff \\
Hospital & ``Universitair Medisch Centrum'', ``UMC'' &  \\
Care Institute & ``Cromhoff'', ``Mgr. Bekkershuis'' &  \\
Organization & ``Ikea'', ``de Vink'', ``de Efteling'' & Generic names: ``bouwmarkt'' \\
Address & ``Van Meeuwenstraat 2, 1234AB Town'', ``Den Bosch'', ``Nieuw-Zeeland'' &  \\
Internal Location & ``8.1'' & Generic locations: ``surgery room'' \\
Age & ``2 jaar en 4 maanden'', ``78'' & \\
Date & ``15-02-19'', ``2019'', ``vrijdag'', ``Zomer '02'', ``herfstvakantie'', ``koningsdag'', & Time of day (14:27) \\
ID & IBAN, license plate, employee number &  \\
SSN/BSN & Burgerservicenummer (BSN) &  \\ \bottomrule
\end{tabular}%
}
\end{table*}
